# Supplementary material for: DiffKG: Knowledge Graph Diffusion Model for Recommendation
Source: arXiv:2312.16890 source file (2023-12-28)
Supplement: Supplementary file 1 [file supplementary.tex]

\section{Supplementary Material}
\balance
\label{sec:supplementary}
